# Supplementary material for: Metropolis-Hastings Data Augmentation for Graph Neural Networks
Source: arXiv:2203.14082 source file (2022-03-26)
Supplement: Supplementary file 2 [file appendix_fig.tex]

\begin{figure}[ht] 
\centering
\includesvg[width=\linewidth]{Analysis/big_sample2.svg}
\caption{
\textbf{Diverse $\G'$ sampled by MH-Aug.} Additional visualizations of subgraphs on CORA dataset. The original graphs $\G$ on the first column are 3-hop ego-graphs from \textcolor[rgb]{0.6,0.5,0.25}{yellow} nodes. The graphs on other columns are augmented graphs drawn by MH-Aug.
}

\label{fig:appendix_ago}
\end{figure}
