# Supplementary material for: Metropolis-Hastings Data Augmentation for Graph Neural Networks
Source: arXiv:2203.14082 source file (2022-03-26)
Supplement: Supplementary file 3 [file suppl.tex]

\begin{figure}[ht] 
\centering
\subfigure[Distribution of $\Delta \G'_{\E}$ w/o Normalization ]{
    \label{subfig:2a}
    \includegraphics[width=\linewidth/2-0.1cm,trim=2cm 0cm 3cm 0cm,clip]{Figures/lam_1_dr.png}%
    % \includegraphics[width=0.8\linewidth]{Figures/lam_1_dr.png}%
    % \includesvg[height=2.8cm]{Figures/lam_0_dr.png}
} % $(\mathbbm{1})_i=1, \ (A\mathbbm{1})_i=4, \ (A^2\mathbbm{1})_i=15$
\hspace{0.cm}

\hspace{-0.35cm}
\subfigure[Distribution of $\Delta \G'_{\E}$ w/ Normalization ]{
    \label{subfig:2b} 
    \includegraphics[width=\linewidth/2-0.1cm,trim=2cm 0cm 3cm 0cm,clip]{Figures/lam_0_dr.png}%
    % \includesvg[width=2.6cm]{Figures/fig2c9.svg}
}

\subfigure[Distribution of $\G'$ w/o Normalization]{
    \label{subfig:2c}
    \includegraphics[width=\linewidth/2-0.3cm,trim=2cm 0cm 3cm 0cm,clip]{Figures/lam_1_sample.png}%
    % \includesvg[height=2.8cm]{Figures/lam_0_dr.png}
} % $(\mathbbm{1})_i=1, \ (A\mathbbm{1})_i=4, \ (A^2\mathbbm{1})_i=15$
\hspace{0.cm}

\hspace{0.cm}
\subfigure[Distribution of $\G'$ w/ Normalization]{
    \label{subfig:2d} 
    \includegraphics[width=\linewidth/2-0.3cm,trim=2cm 0cm 3cm 0cm,clip]{Figures/lam_0_sample.png}%
    % \includesvg[width=2.6cm]{Figures/fig2c9.svg}
}
\hspace{0.2cm}
\caption{\textbf{The effect of normalization term.} The plots above show the distribution of augmented graphs w.r.t. the \textit{change ratio space} $\Delta \G_{\E}$ and the \textit{sample space} $\G$. We conduct the experiments with a uniform distribution as the target distribution. (a) and (b) present the distribution of the \textit{change ratio} $\Delta \G_{\E}$ w/o and w/ normalization. (c) and (d) show the distribution of \textit{sample} $\G$ w/o and w/ normalization. }
% Calculating $\Delta \G'_i$ (\textcolor{orange}{orange}) 
\label{appendix_normalization}
\end{figure}
