# Supplementary material for: Metropolis-Hastings Data Augmentation for Graph Neural Networks
Source: arXiv:2203.14082 source file (2022-03-26)
Supplement: Supplementary file 4 [file calc_accep.tex]

\begin{equation}
\begin{split}
\ln{\alpha} 
&= {\ln{P(\G')} - \ln{P(\G^{(t)})} + \ln{Q(\G^{(t)}|\G')} - \ln{Q(\G'|\G^{(t)})}} \\
&= \lambda_1 \sum_i^{|\V|}{ \left[ - {(\Delta \G'_{i, (\E)} - \mu_\E )^2 \over 2\sigma_\E^2 }  \right]} - \lambda_2 \ln{\binom{|\E|}{|\E| \cdot \Delta \G'_\E}}\\
&\quad  - \lambda_1 \sum_i^{|\V|}{ \left[ - {(\Delta \G^{(t)}_{i, (\E)}- \mu_\E )^2 \over 2\sigma_\E^2 }  \right]} + \lambda_2 \ln{\binom{|\E|}{|\E| \cdot \Delta \G_\E^{(t)}}}\\
  &\quad  + \ln{\TN(\G^{(t)}|\G')} - \ln{\binom{|\E|}{|\E| \cdot \Delta \G_\E^{(t)}}} \\
  &\quad  - \ln{\TN(\G'|\G^{(t)})} + \ln{\binom{|\E|}{|\E| \cdot \Delta \G'_\E}} \\
&=\lambda_1 \sum_i^{|\V|}{ \left[ - {(\Delta \G'_{i, (\E)} - \mu_\E )^2 \over 2\sigma_\E^2 }  \right]} - \lambda_1 \sum_i^{|\V|}{ \left[ - {(\Delta \G^{(t)}_{i, (\E)}- \mu_\E )^2 \over 2\sigma_\E^2 }  \right]} \\
  &\quad  + \ln{\TN(\G^{(t)}|\G')} - \ln{\TN(\G'|\G^{(t)})} \\
  &\quad   + (1 - \lambda_2) \ln{\binom{|\E|}{|\E| \cdot \Delta \G'_\E}} - (1 - \lambda_2) \ln{\binom{|\E|}{|\E| \cdot |\Delta \G_\E^{(t)}|}} \\
&= \lambda_1 \sum_i^{|\V|}{ \left[ - {(\Delta \G'_{i, (\E)}- \mu_\E )^2 \over 2\sigma_\E^2 }  \right]} - \lambda_1 \sum_i^{|\V|}{ \left[ - {(\Delta \G^{(t)}_{i, (\E)}- \mu_\E )^2 \over 2\sigma_\E^2 }  \right]} \\
  &\quad  + \ln{\TN(\G^{(t)}|\G')} - \ln{\TN(\G'|\G^{(t)})} \\
  &\quad  + (1 - \lambda_2) \ln{Beta(|\E| - |\E| \cdot \Delta \G^{(t)} + 1, |\E| \cdot \Delta \G^{(t)} + 1) \over Beta(|\E| - |\E| \cdot \Delta \G' + 1, |\E| \cdot \Delta \G' + 1)},
\end{split}
\end{equation}
