# Supplementary material for: Metropolis-Hastings Data Augmentation for Graph Neural Networks
Source: arXiv:2203.14082 source file (2022-03-26)
Supplement: Supplementary file 5 [file s0.tex]

\section{Reproducibility}

\subsection{Dataset Statistics}
Table \ref{tab:data statistics} summarizes the statistics of five benchmark datasets -- Cora\footnote{Licensed under the Creative Commons Attribution 4.0 International
(CC BY 4.0) Licence}, Citeseer, Amazon Computers, Amazon Photo, and Coauthor CS and two large datasets for additional experiments -- CORA Full and ogbn-arxiv \footnote{
Copyright (c) 2019 OGB Team. Licensed under MIT License}. 
% For CORA Full and ogbn-arxiv dataset, we choose 20 samples per class as a training set. 
% If there is less than 100 nodes in class, we choose training set 20 percent of training nodes. 
We use the same experimental settings on every dataset as semi-supervised graph representation learning~\citep{kipf2016semi,shchur2018pitfalls, hu2020open}.

\begin{table*}[ht] 
    \centering
    \caption{Statistics and details of datasets for node classification.\label{tab:data statistics}}
    \begin{adjustbox}{width=1.0\textwidth}    
    \begin{tabular}{ l  c c c c c c c }
        \toprule
        \multicolumn{1}{ l }{\textbf{Dataset}} & \textbf{\# Nodes} & \textbf{\# Edges} & \textbf{\# Features} & \textbf{\# Classes} & \textbf{\# Train} & \textbf{\# Validation} & \textbf{\# Test} \\ \midrule
        \textbf{CORA}               & 2,708   & 5,429     & 1,433  & 7  & 140 & 500  & 1,000 \\ 
        \textbf{CITESEER}           & 3,327   & 4,732      & 3,703  & 6  & 120 & 500  & 1,000 \\ 
        \textbf{Amazon Computers}   & 13,752  & 245,778    & 767   & 10 & 200 & 300  & 13,252 \\ 
        \textbf{Amazon Photo}       & 7,650   & 119,043    & 745   & 8  & 160 & 240 & 7,250 \\
        \textbf{Coauthor CS}        & 18,333  & 81,894    & 6,805  & 15 & 300 & 450  & 17,583 \\
        \textbf{CORA Full}        & 19,793 & 65,311 & 8,710 & 70 & 1,311 & 1,800 & 16,682 \\
        \textbf{ogbn-arxiv}        & 169,343  & 1,166,243    & 128  & 40 & 90,941 & 29,799 & 48,603 \\
        \bottomrule
    \end{tabular}
    \end{adjustbox}

\end{table*}

\subsection{Implementation Details}
We conduct 10 trials and report the mean and standard deviation over the trials for every experiment. 
In details, we set the number of layers to 2 and the dimensionality of hidden representations to 64 for every datasets, except for the dimensionality of GAT hidden representations to 16 and the number of heads to 8. 
Models are optimized by the Adam~\cite{kingma2015adam} optimizer for 2,000 epochs. As for the baselines, we adopt vanilla models, augmentation-based supervised learning (DropEdge\footnote{Copyright (c) 2019 DropEdge. Licensed under MIT License}~\cite{Rong2020DropEdge:}, AdaEdge~\cite{chen2020measuring}), and semi-supervised learning framework (GAug\footnote{Copyright (c) 2021 Tong Zhao. Licensed under MIT License}~\cite{zhao2020data}, SSL~\cite{zhu2020self}, BVAT\footnote{Copyright (c) 2019 Zhijie. Licensed under MIT License}~\cite{deng2019batch}, UDA*~\cite{xie2020unsupervised}, GraphMix~\cite{verma2019graphmix}). 
We implement the UDA \cite{xie2020unsupervised} which is a semi-supervised framework for consistency training on image recognition and natural language processing. 
Herein we directly implement it for graph structured data and denote with a superscript asterisk `*' in the Table 1 from the main paper. 
For GraphMix with GraphSAGE as base GNNs, we simply adopt the aggregation function of GraphSAGE. The source code for baseline is from the original paper.
Our MH-Aug is implemented in Pytorch~\cite{PyTorch} with the geometric deep learning library Torch-Geometric~\cite{torch_geometric}.  
All the experiments in this paper are conducted on a single Tesla V100 with 16GB memory size. 
As for the software version, we use Python 3.8.3, Pytorch 1.5.0 \footnote{Copyright (c) 2016-Facebook, Inc (Adam Paszke), Licensed under BSD-style license} and Pytorch geometric 1.6.2 \footnote{Copyright (c) 2020 Matthias Fey. Licensed under MIT License}.
\subsection{Hyperparameter Settings}
We delineate additional hyperparameters such as coefficients (\ie, $\alpha_{\E}$, $\beta_{\E}$, $\alpha_{\V}$ and $\beta_{\V}$) of the linear function for standard deviation of the target distribution $\sigma_{(\cdot)}(\epsilon_i) = \alpha_{(\cdot)} * \epsilon_i + \beta_{(\cdot)}$ w.r.t. edges $\E$ and nodes $\V$, respective coefficients of regularization for Kullback-Leibler divergence loss $\gamma_1$ and entropy loss $\gamma_2$, the standard deviation of proposal distribution $\sigma_{\Delta,(\cdot)}$ w.r.t. edges and nodes, and the mean of proposal distribution $\mu_{(\cdot)}$ w.r.t. edges and nodes. 
We empirically perform hyperparameter search for each dataset. 
Table~\ref{table:hyperparams} reports the best hyperparameters of MH-Aug on GCN.

\begin{table}[h] 
  \caption{Hyperparameters of MH-Aug on GCN.} \label{table:table_params}
  \centering
  \label{ablation2}
\setlength{\tabcolsep}{6pt}

\begin{adjustbox}{width=1.0\textwidth}    
  \begin{tabular}{c|ccccc}
    \toprule
    % \multicolumn{7}{c}{asd}\\
    \textbf{Hyperparameters} & \textbf{CORA} & \textbf{CITESEER} & \textbf{Computers} & \textbf{Photo} & \textbf{CS}\\
    \midrule

    $\alpha_{\E}, \beta_{\E}$ 
    % in linear function of the entropy for edges $\sigma_{\E}(\epsilon_i) = \alpha(\epsilon_i) + \beta$ 
    & 10, 1 & 5, 1 & 10, 1 & 10, 1 & 0, 0.1 \\
    $\alpha_{\V}, \beta_{\V}$ 
    % in linear function of the entropy for nodes $\sigma_{\V}(\epsilon_i) = \alpha(\epsilon_i) + \beta$ 
    & 1, 1 & 10, 0.1 & 10, 0.1 & 10, 1 & 5, 0.1 \\
    % Coefficient of regularizer loss $\mathcal{L}_{u}, 
    $\gamma_1$ & 0.5 & 0.2 & 4 & 3 & 0.2 \\
    % Coefficient of regularizer loss $\mathcal{L}_{h}, 
    $\gamma_2$ & 0.5 & 0.5 & 0.4 & 0.5 & 0.4 \\
    % Standard deviance of proposal distribution for edges and nodes 
    $\sigma_{\Delta,(\E)}$,$\sigma_{\Delta,(\V)}$ & 0.1, 0.01 & 0.005, 0.1 & 0.05, 0.01 & 0.01, 0.005 & 0.001, 0.01 \\ 
    % Mean of target distribution for edges and nodes 
    $\mu_{\E}, \mu_{\V}$ & 0.3, 0.7 & 0.2, 0.5 & 0, 0.1 & 0.5, 0 & 0.8, 0.2 \\ 
    % Influence parameter of distribution with the change ratio of ego-graph $\Delta \G_i$ for edges and nodes, 
    $\lambda_1, \lambda_3$ & 5, 1 & 1, 10  & 1, 10 & 1, 10 & 10, 5 \\
    % Influence parameter of normalization term for edges and nodes, 
    $\lambda_2, \lambda_4$ & 0.9999, 0.999 & 0.9999, 0.999 & 0.9999, 0.9999 & 0.9999, 0.9999 & 0.9999, 1\\
%    num_layers = 2
%    emb_dim = 64
%    dropout = 0.5
    
    \bottomrule
  \end{tabular}
\end{adjustbox}
\label{table:hyperparams}
\vspace{-5pt}
\end{table}
