# Supplementary material for: Metropolis-Hastings Data Augmentation for Graph Neural Networks
Source: arXiv:2203.14082 source file (2022-03-26)
Supplement: Supplementary file 6 [file s1.tex]

\section{Proof of Lemma}

\begin{theorem} \textnormal{(Convergence Theorem)} \label{convergence}
Let $X = (X_t)_{t \geq 0}$ be a Markov chain with transition kernel K. If $X$ is \textbf{irreducible}, \textbf{aperiodic} and \textbf{has stationary distribution} $\pi$, then there exist
\begin{equation}
\begin{split}
P(X_t=x|X_0=x_0) \rightarrow \pi(x) \textit{ as } t \rightarrow \infty, \ \textit{for all } x \textit{ and every initial state } x_0.\\
\end{split}
\end{equation}
\end{theorem}

\begin{theorem} \textnormal{(Existence of a Stationary distribution)} \label{existence}
A sufficient but not necessary condition is detailed balance, which requires that each transition ${ x\to x'}$ is reversible.
\end{theorem}

\begin{definition} \label{reversible}
A Markov chain with invariant measure $\pi$ is reversible if and only if
\begin{equation}
    \pi_{i}K_{ij} = \pi_{j}K_{ji}
\end{equation}
for all states i and j, where K is the transition kernel.
\end{definition}

\newenvironment{customthm}[1]
  {\innercustomthm}
  {\endinnercustomthm}
  
\begin{customthm}{3.1}
Let the sequence of augmented graphs $\{\G^{(t)}\}_{0 \leq t\leq T}$ be the Markov chain produced by MH-Aug. If we define the acceptance ratio $\A$ with target distribution $P$ in (4)
and proposal distribution $Q$ in (6),
 the sequence converges to a unique stationary target distribution $P$.
\end{customthm}

\begin{proof}[Proof of Lemma 3.1] By Theorem \ref{convergence}, we can show that MH-Aug converges to the target distribution $P$, if Markov chain of MH-Aug is \textit{irreducible}, \textit{aperiodic} and \textit{has stationary distribution}. First, we will show the existence of stationary distribution by Theorem \ref{existence} and Definition \ref{reversible}. 

The acceptance ratio $\A(\G, \G')$ of Metropolis-Hastings algorithm can be calculated with the proposal distribution $Q$ and the target distribution $P$. Then, the transition kernel $K(\G'|\G)$ can be written as
\begin{equation}
\begin{split}
    K(\G'|\G)=Q(\G'|\G)\A(\G,\G') + \delta_{\G}(\G')r(\G),
\end{split}
\end{equation}
where $r(\G) = 1 - \int \A(\G,s)Q(s|\G)ds$ is the probability of rejecting $\G'$, which is generated by the proposal distribution $Q$ and $\delta_{\G}(\cdot)$ denotes the Dirac delta function located at $\G$. Then, the reversibility can be shown as 
\begin{equation}
\begin{split}
    P(\G)K(\G'|\G) 
    & =  P(\G)Q(\G'|\G)\A(\G,\G') \\
    & = P(\G)Q(\G'|\G)\min\{1, {P(\G')Q(\G|\G') \over P(\G)Q(\G'|\G)}\} \\
    & = \min\{P(\G)Q(\G'|\G), P(\G')Q(\G|\G')\},
\end{split}
\end{equation}

\begin{equation}
\begin{split}
    P(\G')K(\G|\G') 
    & =  P(\G')Q(\G|\G')\A(\G',\G) \\
    & = P(\G')Q(\G|\G')\min\{1, {P(\G)Q(\G'|\G) \over P(\G')Q(\G|\G')}\} \\
    & = \min\{P(\G')Q(\G|\G'), P(\G)Q(\G'|\G)\}.
\end{split}
\end{equation}

\begin{equation}
\begin{split}
     P(\G)K(\G'|\G) = \min\{P(\G)Q(\G'|\G), P(\G')Q(\G|\G')\}
      = P(\G')K(\G|\G').
\end{split}
\end{equation}

By Definition ~\ref{reversible}, $P$ in (4) is reversible and there exists a stationary distribution for Markov chain by Theorem \ref{existence}. 
Note that we do not consider the case of rejection because it is trivial that the detailed balance equation always satisfies when $\G = \G'$. 
Now, we need to show that the Markov chain of MH-Aug is \textit{irreducible} and \textit{aperiodic}. 
The transition kernel $K(\G_j|\G_i)$ for all $i, j$ is defined as:
\begin{equation}
\begin{split}
     K(\G_j|\G_i) 
     & = Q(\G_j|\G_i)\A(\G_i,\G_j) + \delta_{\G_i}(\G_j)r(\G_i).
\end{split}
\end{equation}
Since $Q(\G_j|\G_i)\A(\G_i,\G_j) > 0$  and $\delta_{\G_i}(\G_j)r(\G_i) \geq 0$,
% by Eq. \eqref{eq:P} and \eqref{eq:Q}
Markov chain of MH-Aug has positive probability for all $0 \leq \Delta \G_i \leq 1$ and $0 \leq \Delta \G_j \leq 1$ to reach any range in the support of the proposal distribution. Thus, it is irreducible. % by Def ?.
Similarly, the probability of $\G_i$ to stay at $\G_i$, which can be written as $K(\G_i|\G_i)$, is strictly greater than $0$. Thus, its period is 1, which means that it is aperiodic.
Therefore, by Theorem~\ref{convergence}, MH-Aug converges to the stationary target distribution $P$.
\end{proof}
