# Supplementary material for: Metropolis-Hastings Data Augmentation for Graph Neural Networks
Source: arXiv:2203.14082 source file (2022-03-26)
Supplement: Supplementary file 7 [file s2_0.tex]

\section{Additional Experiments}
\subsection{Further Visualizations of Augmented Graphs by MH-Aug} %Examples of Augmented Graphs sampled by MH-Aug
\label{sec:supp-samples}
\begin{figure}[ht] 
\centering
\includesvg[width=\linewidth]{Analysis/big_sample2.svg}
\caption{
\textbf{Diverse $\G'$ sampled by MH-Aug.} Additional visualizations of subgraphs on CORA dataset. The original graphs $\G$ on the first column are 3-hop ego-graphs from \textcolor[rgb]{0.6,0.5,0.25}{yellow} nodes. The graphs on other columns are augmented graphs drawn by MH-Aug.
}

\label{fig:appendix_ago}
\end{figure}

As shown in Figure~\ref{fig:appendix_ago}, we provide more visualizations of augmented graphs by MH-Aug with various settings. 
Original samples in the first column are a 3-hop ego-graph from CORA and the corresponding augmented samples in the other columns are generated from original samples.
Augmented samples are drawn from three different target distributions as same as the main paper. 

We only consider the edge drop, not the node drop in this visualization for simplicity and fix the number of dropped edges $\Delta \G'_{\E}$ to evaluate the effect of $\mu_{\E}$ and $\sigma_{\E}$ in the target distribution. 
Mini maps represent the Edge-Drop probability directly calculated from $P$.  

In Figure \ref{fig:appendix_ago}, we can verify two things.
First, MH-Aug samples the augmented graphs following the target distribution. 
If the Edge-Drop probability of a specific edge is high according to the target distribution (red), then the corresponding edge tends to be dropped in the augmented graph drawn by MH-Aug.
Second, MH-Aug controls the strength and diversity of augmentation with $\mu_{\E}$ and $\sigma_{\E}$. When $\mu_{\E}$, which controls the expected augmentation strength, is large, \eg,  $\mu_{\E}=1,\sigma_{\E}=0.05$, more important edges (\eg, edges acting as bridges between hub nodes) tend to be dropped. 
Conversely, when $\mu_{\E}$ is small, \eg,  $\mu_{\E}=0,\sigma_{\E}=0.05$, relatively unimportant edges are likely to be dropped. 
It verifies that we can control the strength of the augmentation by $\mu_{\E}$ even with the same number of dropped edges.
Moreover, by adjusting $\sigma_{\E}$, we can control the diversity of augmentation. The mini map in the fourth column of Figure~\ref{fig:appendix_ago} shows that if $\sigma_\E$ increases, the Edge-Drop probability of all edges becomes uniform, \ie, MH-Aug subsumes DropEdge as a special case. 
Thus, if we set $\sigma_\E$ to be large, MH-Aug generates samples with diverse augmentation strength. 
In sum, the ego-graph perspective enables the explicit control of augmentation strength and diversity to make an advanced augmentation.

\subsection{Ablation Study}

As an ablation study, we conduct experiments with MH-Aug (w/o Reg), our framework trained in the supervised setting, MH-Aug (w/o Normalization), which has the target distribution without normalization term (\ie, $\lambda_2=0$ and $\lambda_4=0$) and MH-Aug (w/o Entropy), which trained in the semi-supervised setting but without entropy loss $\mathcal{L}_h$. Table \ref{table:ablation} shows the contribution of each component in our framework. 
The results present the importance of each component and it is worth noting that normalization is \textit{crucial} to generate desired samples. On Computers, we observed that MH-Aug (w/o Normalization) underperforms the vanilla supervised training.  

\begin{table}[ht] 
  \caption{Ablation study of MH-Aug with GCN.} \label{table:ablation}
  \centering
\setlength{\tabcolsep}{6pt}

\begin{adjustbox}{width=1.0\textwidth}    
  \begin{tabular}{l|ccccc}
    \toprule
    % \multicolumn{7}{c}{asd}\\
    \textbf{Methods} & \textbf{CORA} & \textbf{CITESEER} & \textbf{Computers} & \textbf{Photo} & \textbf{CS}\\
    \midrule
    
    % \multirow{3}{*}{}
    Vanilla & 81.54{\scriptsize$\pm$0.76} & 71.64{\scriptsize$\pm$0.31} & 79.68{\scriptsize$\pm$2.16} & 89.02{\scriptsize$\pm$1.49} & 91.45{\scriptsize$\pm$0.28} \\
    MH-Aug (w/o Reg) & 83.55{\scriptsize$\pm$0.34} & 72.96{\scriptsize$\pm$0.48} & 80.95{\scriptsize$\pm$2.03} & 89.65{\scriptsize$\pm$1.67} & 91.81{\scriptsize$\pm$0.33} \\
    MH-Aug (w/o Normalization)  & 82.88{\scriptsize$\pm$0.62} & 74.81{\scriptsize$\pm$0.48} & 73.49{\scriptsize$\pm$2.20} & 90.75{\scriptsize$\pm$1.41} & 92.45{\scriptsize$\pm$0.62} \\
    MH-Aug (w/o Entropy)  & 82.53{\scriptsize$\pm$0.49} & 71.63{\scriptsize$\pm$0.57} & 80.88{\scriptsize$\pm$1.90} & 89.82{\scriptsize$\pm$1.63} & 91.96{\scriptsize$\pm$0.60} \\
    MH-Aug & \textbf{85.16{\scriptsize$\pm$0.35}} & \textbf{75.49{\scriptsize$\pm$0.29}} & \textbf{82.80{\scriptsize$\pm$2.08}} & \textbf{90.87{\scriptsize$\pm$1.49}} & \textbf{92.60{\scriptsize$\pm$0.43}} \\
    
    \bottomrule
  \end{tabular}
\end{adjustbox}
\vspace{-5pt}
\end{table}

\subsection{Results on Large Datasets}
We also evaluate our framework on two relatively large datasets -- CORA Full and ogbn-arxiv. Cora-Full is proposed in \cite{shchur2018pitfalls} and ogbn-arxiv is in \cite{hu2020open}. We randomly select $K \in \{10, 20\}$ nodes per class from the training set. We conduct 10 trials for CORA Full and 3 trials for ogbn-arxiv and report the mean and standard deviation over the trials for every experiment. The results are presented in Table \ref{table:large}. We can observe that MH-Aug outperforms overall base model (\ie, GCN\footnote{Copyright (c) 2016 Thomas Kipf. Licensed under MIT License}, GraphSAGE\footnote{Copyright (c) 2017 William L. Hamilton, Rex Ying. Licensed under MIT License} and GAT\footnote{Copyright (c) 2018 Petar Veličković. Licensed under MIT License}). 
% +) results
Our framework surpasses the vanilla models on both ogbn-arxiv and CORA Full datasets. When K=10, MH-Aug achieves the improvement of 6.83$\%$ against the vanilla model on average. With 10 labeled data per class, our method provides 6.25$\%$ performance improvement compared to the vanilla model on average.

\begin{table}[h] 
  \caption{Node classification results on large datasets with K labeled data per class.} \label{table:large}
  \centering
  \label{ablation2}
\begin{adjustbox}{width=11cm}     
\begin{tabular}{cl|cccc}
\toprule
\multirow{2}{*}{\textbf{BaseGNNs}} & \multirow{2}{*}{\textbf{Method}} &  \multicolumn{2}{c}{\textbf{ogbn-arxiv}} &  \multicolumn{2}{c}{\textbf{CORA Full}} \\
% \cmidrule{3-4}
 &  & K=10 & K=20 & K=10 & K=20\\
\midrule
\multirow{2}{*}{\textbf{GCN}}
& Vanilla   & 47.83{\scriptsize$\pm$1.13} & 54.17{\scriptsize$\pm$1.80} & 54.14{\scriptsize$\pm$ 0.72} & 59.99{\scriptsize$\pm$ 0.39}  \\
& MH-Aug & \textbf{56.19{\scriptsize$\pm$0.44}} & \textbf{61.22{\scriptsize$\pm$0.33}}& \textbf{56.27{\scriptsize$\pm$1.97}} & \textbf{62.79{\scriptsize$\pm$0.49}}   \\
\midrule
\multirow{2}{*}{\textbf{GraphSAGE}}
& Vanilla  & 42.35{\scriptsize$\pm$1.52} & 49.19{\scriptsize$\pm$0.42}  & 52.31{\scriptsize$\pm$ 1.18} & 58.85{\scriptsize$\pm$ 0.43}  \\
& MH-Aug & \textbf{59.01{\scriptsize$\pm$0.28}} & \textbf{61.09{\scriptsize$\pm$0.67}} & \textbf{52.46{\scriptsize$\pm$0.88}} & \textbf{62.57{\scriptsize$\pm$0.73}}  \\

\bottomrule
\end{tabular}
\end{adjustbox}

\end{table} 
