# Supplementary material for: Metropolis-Hastings Data Augmentation for Graph Neural Networks
Source: arXiv:2203.14082 source file (2022-03-26)
Supplement: Supplementary file 8 [file s2_1.examples.tex]

\subsection{Further Visualizations of Augmented Graphs by MH-Aug} %Examples of Augmented Graphs sampled by MH-Aug
\label{sec:supp-samples}
\begin{figure}[ht] 
\centering
\includesvg[width=\linewidth]{Analysis/big_sample2.svg}
\caption{
\textbf{Diverse $\G'$ sampled by MH-Aug.} Additional visualizations of subgraphs on CORA dataset. The original graphs $\G$ on the first column are 3-hop ego-graphs from \textcolor[rgb]{0.6,0.5,0.25}{yellow} nodes. The graphs on other columns are augmented graphs drawn by MH-Aug.
}

\label{fig:appendix_ago}
\end{figure}

As shown in Figure~\ref{fig:appendix_ago}, we provide more visualizations of augmented graphs by MH-Aug with various settings. 
Original samples in the first column are a 3-hop ego-graph from CORA and the corresponding augmented samples in the other columns are generated from original samples.
Augmented samples are drawn from three different target distributions as same as the main paper. 

We only consider the edge drop, not the node drop in this visualization for simplicity and fix the number of dropped edges $\Delta \G'_{\E}$ to evaluate the effect of $\mu_{\E}$ and $\sigma_{\E}$ in the target distribution. 
Mini maps represent the Edge-Drop probability directly calculated from $P$.  

In Figure \ref{fig:appendix_ago}, we can verify two things.
First, MH-Aug samples the augmented graphs following the target distribution. 
If the Edge-Drop probability of a specific edge is high according to the target distribution (red), then the corresponding edge tends to be dropped in the augmented graph drawn by MH-Aug.
Second, MH-Aug controls the strength and diversity of augmentation with $\mu_{\E}$ and $\sigma_{\E}$. When $\mu_{\E}$, which controls the expected augmentation strength, is large, \eg,  $\mu_{\E}=1,\sigma_{\E}=0.05$, more important edges (\eg, edges acting as bridges between hub nodes) tend to be dropped. 
Conversely, when $\mu_{\E}$ is small, \eg,  $\mu_{\E}=0,\sigma_{\E}=0.05$, relatively unimportant edges are likely to be dropped. 
It verifies that we can control the strength of the augmentation by $\mu_{\E}$ even with the same number of dropped edges.
Moreover, by adjusting $\sigma_{\E}$, we can control the diversity of augmentation. The mini map in the fourth column of Figure~\ref{fig:appendix_ago} shows that if $\sigma_\E$ increases, the Edge-Drop probability of all edges becomes uniform, \ie, MH-Aug subsumes DropEdge as a special case. 
Thus, if we set $\sigma_\E$ to be large, MH-Aug generates samples with diverse augmentation strength. 
In sum, the ego-graph perspective enables the explicit control of augmentation strength and diversity to make an advanced augmentation.
