# Supplementary material for: Metropolis-Hastings Data Augmentation for Graph Neural Networks
Source: arXiv:2203.14082 source file (2022-03-26)
Supplement: Supplementary file 11 [file s3_0.tex]

\section{Further Discussion}
\subsection{Normalization Term of Target Distribution}
As mentioned in Figure 4 of the main paper, the normalization in the target distribution $P$ by the number of possible augmented graphs corresponding to the same change ratio, $\binom{|\E|}{|\E|\cdot\Delta \G'_{\E}}$, is crucial to generate ego-graphs with the desired ego-graph change ratio $\mu_{\E}$. 
In this part, we simulate the sampling process of MH-Aug with a simple distribution (\ie, uniform distribution) as the target distribution. 
To examine the necessity of normalization, we observe the distribution of augmented graphs w.r.t. the \textit{change ratio space}, \ie, $\Delta \G'_{\E}$ (the first row in Figure \ref{appendix_normalization}) and the \textit{sample space}, \ie, $\G'$ (the second row in Figure \ref{appendix_normalization}). If we define the target distribution without normalization, it follows uniform distribution aspect to the \textit{sample space} as shown in Figure \ref{subfig:2c}. However, in the perspective of the \textit{change ratio space}, the change ratio is concentrated on 0.5 as described in Figure \ref{subfig:2a}. This is natural, as the number of possible subgraphs on 0.5 change ratio $\binom{|\E|}{|\E|\cdot 0.5}$ is overwhelmingly large compared to the other change ratios.
Since our desired target distribution is related to the change ratio $\Delta \G'_{\E}$, we need to generate samples that follow target distribution (\eg, uniform distribution) in terms of the \textit{change ratio space}. By adopting normalization with the number of possible augmented graphs corresponding to the same change ratio, MH-Aug generates augmented graphs following the target distribution in the perspective of the \textit{change ratio space} as shown in Figure \ref{subfig:2b}. Note that, if we draw the same number of subgraphs for each change ratio, it is inevitable to sample the identical subgraphs that have extreme change ratios. For instance, Figure \ref{subfig:2d} shows that the original graph ($\Delta \G'_{\E}=0$) and the graph without any edge ($\Delta \G'_{\E}=1$) are most frequently sampled since they have only one possible subgraph with the same change ratio.
\begin{figure}[ht] 
\centering
\subfigure[Distribution of $\Delta \G'_{\E}$ w/o Normalization ]{
    \label{subfig:2a}
    \includegraphics[width=\linewidth/2-0.1cm,trim=2cm 0cm 3cm 0cm,clip]{Figures/lam_1_dr.png}%
    % \includegraphics[width=0.8\linewidth]{Figures/lam_1_dr.png}%
    % \includesvg[height=2.8cm]{Figures/lam_0_dr.png}
} % $(\mathbbm{1})_i=1, \ (A\mathbbm{1})_i=4, \ (A^2\mathbbm{1})_i=15$
\hspace{0.cm}

\hspace{-0.35cm}
\subfigure[Distribution of $\Delta \G'_{\E}$ w/ Normalization ]{
    \label{subfig:2b} 
    \includegraphics[width=\linewidth/2-0.1cm,trim=2cm 0cm 3cm 0cm,clip]{Figures/lam_0_dr.png}%
    % \includesvg[width=2.6cm]{Figures/fig2c9.svg}
}

\subfigure[Distribution of $\G'$ w/o Normalization]{
    \label{subfig:2c}
    \includegraphics[width=\linewidth/2-0.3cm,trim=2cm 0cm 3cm 0cm,clip]{Figures/lam_1_sample.png}%
    % \includesvg[height=2.8cm]{Figures/lam_0_dr.png}
} % $(\mathbbm{1})_i=1, \ (A\mathbbm{1})_i=4, \ (A^2\mathbbm{1})_i=15$
\hspace{0.cm}

\hspace{0.cm}
\subfigure[Distribution of $\G'$ w/ Normalization]{
    \label{subfig:2d} 
    \includegraphics[width=\linewidth/2-0.3cm,trim=2cm 0cm 3cm 0cm,clip]{Figures/lam_0_sample.png}%
    % \includesvg[width=2.6cm]{Figures/fig2c9.svg}
}
\hspace{0.2cm}
\caption{\textbf{The effect of normalization term.} The plots above show the distribution of augmented graphs w.r.t. the \textit{change ratio space} $\Delta \G_{\E}$ and the \textit{sample space} $\G$. We conduct the experiments with a uniform distribution as the target distribution. (a) and (b) present the distribution of the \textit{change ratio} $\Delta \G_{\E}$ w/o and w/ normalization. (c) and (d) show the distribution of \textit{sample} $\G$ w/o and w/ normalization. }
% Calculating $\Delta \G'_i$ (\textcolor{orange}{orange}) 
\label{appendix_normalization}
\end{figure}

\subsection{Calculation of Acceptance Ratio}
In Metropolis-Hastings algorithm, the acceptance ratio $\A$ is given as:
\begin{equation} \label{eq:acceptance ratio}
% \begin{split}
\A  = \min \left \{1,{P(\G')Q(\G^{(t)}|\G') \over P(\G^{(t)})Q(\G'|\G^{(t)})}\right \}. 
% \end{split}
\end{equation}
Here, we only consider the augmentation of edge for simplicity. The target distribution of MH-Aug can be written as follow:
\begin{equation}
    \begin{split}
    P_{\E}(\G') \propto \left[ \prod_{i}^{|\V|} \exp{\left( - {(\Delta \G'_{i, (\E)}- \mu_{\E})^2 \over 2\sigma_{\E}^2 } \right)} \right]^{\lambda_1} \cdot \left[ 1 \over \binom{|\E|}{|\E|\cdot\Delta \G'_\E} \right]^{\lambda_2}, \\
    \ln{P_{\E}(\G')} \propto \lambda_1 \sum_i^{|\V|}{ \left[ - {(\Delta \G'_{i, (\E)} - \mu_{\E} )^2 \over 2\sigma_{\E}^2 }  \right]} - \lambda_2 \ln{\binom{|\E|}{|\E|\cdot\Delta \G'_{\E}}} 
    \end{split}
\end{equation}
The proposal distribution of MH-Aug can be written as:
\begin{equation}
\begin{split}
    Q_\E(\G^{(t)}|\G') \propto {\phi(\xi^{(t)}_{\E}) \over \Phi(\beta'_{\E}) - \Phi(\alpha'_{\E})} \cdot {1 \over \binom{|\E|}{|\E|\cdot\Delta \G'_{\E}}}, \\
    \ln{Q_\E(\G^{(t)}|\G')} \propto \ln{\phi(\xi^{(t)}_{\E}) \over \Phi(\beta'_{\E}) - \Phi(\alpha'_{\E})} - \ln{\binom{|\E|}{|\E|\cdot\Delta \G^{(t)}_{\E}}},
\end{split}
\end{equation}
where $\alpha'_{\E} = {a - \Delta \G'_{\E} \over \sigma_{\Delta}}, \ \beta'_{\E} = {b - \Delta \G'_{\E} \over \sigma_{\Delta}}, \ \xi^{(t)}_{\E} = {\Delta \G^{(t)}_{\E} - \Delta \G'_{\E} \over \sigma_{\Delta}},\phi(x) = {1\over \sqrt{2\pi}}\exp(-{1 \over 2} x^2)$ as the probability density function of the standard normal distribution and  $\Phi(x)= {1 \over 2}(1+erf({x \over \sqrt{2}}))$ as its cumulative distribution function. 
% $a, b$ : range of truncated $\G$
% $\sigma_{\Delta}$ : standard deviation of truncated $\G$
For simplicity, we denote the first term (\ie, truncated Gaussian given $\mu=\G'$, $\sigma=\sigma_{\Delta}$, and range=[a,b])  as $\TN(\G^{(t)};\G',\sigma_{\Delta},a,b) $ where a and b are the range of truncated Gaussian distribution and they are fixed to 0 and 1 respectively. Then, $\alpha = {{P(\G')Q(\G^{(t)}|\G') \over P(\G^{(t)})Q(\G'|\G^{(t)})}}$ can be calculated as follow:

\begin{equation}
\begin{split}
\ln{\alpha} 
&= {\ln{P(\G')} - \ln{P(\G^{(t)})} + \ln{Q(\G^{(t)}|\G')} - \ln{Q(\G'|\G^{(t)})}} \\
&= \lambda_1 \sum_i^{|\V|}{ \left[ - {(\Delta \G'_{i, (\E)} - \mu_\E )^2 \over 2\sigma_\E^2 }  \right]} - \lambda_2 \ln{\binom{|\E|}{|\E| \cdot \Delta \G'_\E}}\\
&\quad  - \lambda_1 \sum_i^{|\V|}{ \left[ - {(\Delta \G^{(t)}_{i, (\E)}- \mu_\E )^2 \over 2\sigma_\E^2 }  \right]} + \lambda_2 \ln{\binom{|\E|}{|\E| \cdot \Delta \G_\E^{(t)}}}\\
  &\quad  + \ln{\TN(\G^{(t)}|\G')} - \ln{\binom{|\E|}{|\E| \cdot \Delta \G_\E^{(t)}}} \\
  &\quad  - \ln{\TN(\G'|\G^{(t)})} + \ln{\binom{|\E|}{|\E| \cdot \Delta \G'_\E}} \\
&=\lambda_1 \sum_i^{|\V|}{ \left[ - {(\Delta \G'_{i, (\E)} - \mu_\E )^2 \over 2\sigma_\E^2 }  \right]} - \lambda_1 \sum_i^{|\V|}{ \left[ - {(\Delta \G^{(t)}_{i, (\E)}- \mu_\E )^2 \over 2\sigma_\E^2 }  \right]} \\
  &\quad  + \ln{\TN(\G^{(t)}|\G')} - \ln{\TN(\G'|\G^{(t)})} \\
  &\quad   + (1 - \lambda_2) \ln{\binom{|\E|}{|\E| \cdot \Delta \G'_\E}} - (1 - \lambda_2) \ln{\binom{|\E|}{|\E| \cdot |\Delta \G_\E^{(t)}|}} \\
&= \lambda_1 \sum_i^{|\V|}{ \left[ - {(\Delta \G'_{i, (\E)}- \mu_\E )^2 \over 2\sigma_\E^2 }  \right]} - \lambda_1 \sum_i^{|\V|}{ \left[ - {(\Delta \G^{(t)}_{i, (\E)}- \mu_\E )^2 \over 2\sigma_\E^2 }  \right]} \\
  &\quad  + \ln{\TN(\G^{(t)}|\G')} - \ln{\TN(\G'|\G^{(t)})} \\
  &\quad  + (1 - \lambda_2) \ln{Beta(|\E| - |\E| \cdot \Delta \G^{(t)} + 1, |\E| \cdot \Delta \G^{(t)} + 1) \over Beta(|\E| - |\E| \cdot \Delta \G' + 1, |\E| \cdot \Delta \G' + 1)},
\end{split}
\end{equation}

where $Beta(\cdot)$ is the beta function. Since the calculation of a combination might cause a numerical error, in our implementation we adopt \textit{betaln} in scipy \cite{scipy} instead of the combination. It can be calculated similarly in the case of considering both edge and node augmentation. 
\subsection{Negative Societal Impacts and Limitations}

\paragraph{Negative Societal Impacts.} 
MH-AUG is a generic semi-supervised learning framework with a novel augmentation method.
We believe that there is no direct negative societal impact of this work.
However, like other augmentation methods or GNN models for graph-structured data, our generic framework can be used for malicious activities.
GNNs are capable to extract uncharted knowledge from the graph data (\eg, a graph with private information extracted from social media).
Through the misappropriation of graphs with sensitive information, it might incite or manipulate public opinion.
To mitigate the potential problems, illegal data collection should be prevented and it is encouraged to put the dataset under rigorous scrutiny before the release.
% In this paper, we address the problem of weak-generalization of Graph Neural Networks. We study augmentation for GNNs on graph-structured data, so we have some issues that graph-structured data and GNNs intrinsically have. Since graph data is provided by a certain community, it should be noted that the data itself might be biased depending on the community. In addition, since GNNs use surrounding neighbors' information in the process of aggregation, there may be security issues of data privacy such as their relationship and the property. 

\paragraph{Limitations.} Since we adopt the MCMC sampling for augmentation, our method also has the burn-in issue that is common in MCMC methods. To mitigate this problem, we start from the original graph which is at an area with a high probability density. But, for an extreme target distribution, this initialization might not be sufficient to resolve the burn-in issue and better initialization needs to be studied. 
In addition, we propose a simple target distribution based on Gaussian distribution with a normalization. However, there might be more ideal target distributions for effective augmentation. These are left for future works.
