# Supplementary material for: Metropolis-Hastings Data Augmentation for Graph Neural Networks
Source: arXiv:2203.14082 source file (2022-03-26)
Supplement: Supplementary file 12 [file s3_1.normalization.tex]

\subsection{Normalization Term of Target Distribution}
As mentioned in Figure 4 of the main paper, the normalization in the target distribution $P$ by the number of possible augmented graphs corresponding to the same change ratio, $\binom{|\E|}{|\E|\cdot\Delta \G'_{\E}}$, is crucial to generate ego-graphs with the desired ego-graph change ratio $\mu_{\E}$. 
In this part, we simulate the sampling process of MH-Aug with a simple distribution (\ie, uniform distribution) as the target distribution. 
To examine the necessity of normalization, we observe the distribution of augmented graphs w.r.t. the \textit{change ratio space}, \ie, $\Delta \G'_{\E}$ (the first row in Figure \ref{appendix_normalization}) and the \textit{sample space}, \ie, $\G'$ (the second row in Figure \ref{appendix_normalization}). If we define the target distribution without normalization, it follows uniform distribution aspect to the \textit{sample space} as shown in Figure \ref{subfig:2c}. However, in the perspective of the \textit{change ratio space}, the change ratio is concentrated on 0.5 as described in Figure \ref{subfig:2a}. This is natural, as the number of possible subgraphs on 0.5 change ratio $\binom{|\E|}{|\E|\cdot 0.5}$ is overwhelmingly large compared to the other change ratios.
Since our desired target distribution is related to the change ratio $\Delta \G'_{\E}$, we need to generate samples that follow target distribution (\eg, uniform distribution) in terms of the \textit{change ratio space}. By adopting normalization with the number of possible augmented graphs corresponding to the same change ratio, MH-Aug generates augmented graphs following the target distribution in the perspective of the \textit{change ratio space} as shown in Figure \ref{subfig:2b}. Note that, if we draw the same number of subgraphs for each change ratio, it is inevitable to sample the identical subgraphs that have extreme change ratios. For instance, Figure \ref{subfig:2d} shows that the original graph ($\Delta \G'_{\E}=0$) and the graph without any edge ($\Delta \G'_{\E}=1$) are most frequently sampled since they have only one possible subgraph with the same change ratio.
\begin{figure}[ht] 
\centering
\subfigure[Distribution of $\Delta \G'_{\E}$ w/o Normalization ]{
    \label{subfig:2a}
    \includegraphics[width=\linewidth/2-0.1cm,trim=2cm 0cm 3cm 0cm,clip]{Figures/lam_1_dr.png}%
    % \includegraphics[width=0.8\linewidth]{Figures/lam_1_dr.png}%
    % \includesvg[height=2.8cm]{Figures/lam_0_dr.png}
} % $(\mathbbm{1})_i=1, \ (A\mathbbm{1})_i=4, \ (A^2\mathbbm{1})_i=15$
\hspace{0.cm}

\hspace{-0.35cm}
\subfigure[Distribution of $\Delta \G'_{\E}$ w/ Normalization ]{
    \label{subfig:2b} 
    \includegraphics[width=\linewidth/2-0.1cm,trim=2cm 0cm 3cm 0cm,clip]{Figures/lam_0_dr.png}%
    % \includesvg[width=2.6cm]{Figures/fig2c9.svg}
}

\subfigure[Distribution of $\G'$ w/o Normalization]{
    \label{subfig:2c}
    \includegraphics[width=\linewidth/2-0.3cm,trim=2cm 0cm 3cm 0cm,clip]{Figures/lam_1_sample.png}%
    % \includesvg[height=2.8cm]{Figures/lam_0_dr.png}
} % $(\mathbbm{1})_i=1, \ (A\mathbbm{1})_i=4, \ (A^2\mathbbm{1})_i=15$
\hspace{0.cm}

\hspace{0.cm}
\subfigure[Distribution of $\G'$ w/ Normalization]{
    \label{subfig:2d} 
    \includegraphics[width=\linewidth/2-0.3cm,trim=2cm 0cm 3cm 0cm,clip]{Figures/lam_0_sample.png}%
    % \includesvg[width=2.6cm]{Figures/fig2c9.svg}
}
\hspace{0.2cm}
\caption{\textbf{The effect of normalization term.} The plots above show the distribution of augmented graphs w.r.t. the \textit{change ratio space} $\Delta \G_{\E}$ and the \textit{sample space} $\G$. We conduct the experiments with a uniform distribution as the target distribution. (a) and (b) present the distribution of the \textit{change ratio} $\Delta \G_{\E}$ w/o and w/ normalization. (c) and (d) show the distribution of \textit{sample} $\G$ w/o and w/ normalization. }
% Calculating $\Delta \G'_i$ (\textcolor{orange}{orange}) 
\label{appendix_normalization}
\end{figure}
