# Supplementary material for: Metropolis-Hastings Data Augmentation for Graph Neural Networks
Source: arXiv:2203.14082 source file (2022-03-26)
Supplement: Supplementary file 13 [file s3_2.acceptance.tex]

\subsection{Calculation of Acceptance Ratio}
In Metropolis-Hastings algorithm, the acceptance ratio $\A$ is given as:
\begin{equation} \label{eq:acceptance ratio}
% \begin{split}
\A  = \min \left \{1,{P(\G')Q(\G^{(t)}|\G') \over P(\G^{(t)})Q(\G'|\G^{(t)})}\right \}. 
% \end{split}
\end{equation}
Here, we only consider the augmentation of edge for simplicity. The target distribution of MH-Aug can be written as follow:
\begin{equation}
    \begin{split}
    P_{\E}(\G') \propto \left[ \prod_{i}^{|\V|} \exp{\left( - {(\Delta \G'_{i, (\E)}- \mu_{\E})^2 \over 2\sigma_{\E}^2 } \right)} \right]^{\lambda_1} \cdot \left[ 1 \over \binom{|\E|}{|\E|\cdot\Delta \G'_\E} \right]^{\lambda_2}, \\
    \ln{P_{\E}(\G')} \propto \lambda_1 \sum_i^{|\V|}{ \left[ - {(\Delta \G'_{i, (\E)} - \mu_{\E} )^2 \over 2\sigma_{\E}^2 }  \right]} - \lambda_2 \ln{\binom{|\E|}{|\E|\cdot\Delta \G'_{\E}}} 
    \end{split}
\end{equation}
The proposal distribution of MH-Aug can be written as:
\begin{equation}
\begin{split}
    Q_\E(\G^{(t)}|\G') \propto {\phi(\xi^{(t)}_{\E}) \over \Phi(\beta'_{\E}) - \Phi(\alpha'_{\E})} \cdot {1 \over \binom{|\E|}{|\E|\cdot\Delta \G'_{\E}}}, \\
    \ln{Q_\E(\G^{(t)}|\G')} \propto \ln{\phi(\xi^{(t)}_{\E}) \over \Phi(\beta'_{\E}) - \Phi(\alpha'_{\E})} - \ln{\binom{|\E|}{|\E|\cdot\Delta \G^{(t)}_{\E}}},
\end{split}
\end{equation}
where $\alpha'_{\E} = {a - \Delta \G'_{\E} \over \sigma_{\Delta}}, \ \beta'_{\E} = {b - \Delta \G'_{\E} \over \sigma_{\Delta}}, \ \xi^{(t)}_{\E} = {\Delta \G^{(t)}_{\E} - \Delta \G'_{\E} \over \sigma_{\Delta}},\phi(x) = {1\over \sqrt{2\pi}}\exp(-{1 \over 2} x^2)$ as the probability density function of the standard normal distribution and  $\Phi(x)= {1 \over 2}(1+erf({x \over \sqrt{2}}))$ as its cumulative distribution function. 
% $a, b$ : range of truncated $\G$
% $\sigma_{\Delta}$ : standard deviation of truncated $\G$
For simplicity, we denote the first term (\ie, truncated Gaussian given $\mu=\G'$, $\sigma=\sigma_{\Delta}$, and range=[a,b])  as $\TN(\G^{(t)};\G',\sigma_{\Delta},a,b) $ where a and b are the range of truncated Gaussian distribution and they are fixed to 0 and 1 respectively. Then, $\alpha = {{P(\G')Q(\G^{(t)}|\G') \over P(\G^{(t)})Q(\G'|\G^{(t)})}}$ can be calculated as follow:

\begin{equation}
\begin{split}
\ln{\alpha} 
&= {\ln{P(\G')} - \ln{P(\G^{(t)})} + \ln{Q(\G^{(t)}|\G')} - \ln{Q(\G'|\G^{(t)})}} \\
&= \lambda_1 \sum_i^{|\V|}{ \left[ - {(\Delta \G'_{i, (\E)} - \mu_\E )^2 \over 2\sigma_\E^2 }  \right]} - \lambda_2 \ln{\binom{|\E|}{|\E| \cdot \Delta \G'_\E}}\\
&\quad  - \lambda_1 \sum_i^{|\V|}{ \left[ - {(\Delta \G^{(t)}_{i, (\E)}- \mu_\E )^2 \over 2\sigma_\E^2 }  \right]} + \lambda_2 \ln{\binom{|\E|}{|\E| \cdot \Delta \G_\E^{(t)}}}\\
  &\quad  + \ln{\TN(\G^{(t)}|\G')} - \ln{\binom{|\E|}{|\E| \cdot \Delta \G_\E^{(t)}}} \\
  &\quad  - \ln{\TN(\G'|\G^{(t)})} + \ln{\binom{|\E|}{|\E| \cdot \Delta \G'_\E}} \\
&=\lambda_1 \sum_i^{|\V|}{ \left[ - {(\Delta \G'_{i, (\E)} - \mu_\E )^2 \over 2\sigma_\E^2 }  \right]} - \lambda_1 \sum_i^{|\V|}{ \left[ - {(\Delta \G^{(t)}_{i, (\E)}- \mu_\E )^2 \over 2\sigma_\E^2 }  \right]} \\
  &\quad  + \ln{\TN(\G^{(t)}|\G')} - \ln{\TN(\G'|\G^{(t)})} \\
  &\quad   + (1 - \lambda_2) \ln{\binom{|\E|}{|\E| \cdot \Delta \G'_\E}} - (1 - \lambda_2) \ln{\binom{|\E|}{|\E| \cdot |\Delta \G_\E^{(t)}|}} \\
&= \lambda_1 \sum_i^{|\V|}{ \left[ - {(\Delta \G'_{i, (\E)}- \mu_\E )^2 \over 2\sigma_\E^2 }  \right]} - \lambda_1 \sum_i^{|\V|}{ \left[ - {(\Delta \G^{(t)}_{i, (\E)}- \mu_\E )^2 \over 2\sigma_\E^2 }  \right]} \\
  &\quad  + \ln{\TN(\G^{(t)}|\G')} - \ln{\TN(\G'|\G^{(t)})} \\
  &\quad  + (1 - \lambda_2) \ln{Beta(|\E| - |\E| \cdot \Delta \G^{(t)} + 1, |\E| \cdot \Delta \G^{(t)} + 1) \over Beta(|\E| - |\E| \cdot \Delta \G' + 1, |\E| \cdot \Delta \G' + 1)},
\end{split}
\end{equation}

where $Beta(\cdot)$ is the beta function. Since the calculation of a combination might cause a numerical error, in our implementation we adopt \textit{betaln} in scipy \cite{scipy} instead of the combination. It can be calculated similarly in the case of considering both edge and node augmentation.
