# Supplementary material for: Metropolis-Hastings Data Augmentation for Graph Neural Networks
Source: arXiv:2203.14082 source file (2022-03-26)
Supplement: Supplementary file 14 [file s3_3.limitations.tex]

\subsection{Negative Societal Impacts and Limitations}

\paragraph{Negative Societal Impacts.} 
MH-AUG is a generic semi-supervised learning framework with a novel augmentation method.
We believe that there is no direct negative societal impact of this work.
However, like other augmentation methods or GNN models for graph-structured data, our generic framework can be used for malicious activities.
GNNs are capable to extract uncharted knowledge from the graph data (\eg, a graph with private information extracted from social media).
Through the misappropriation of graphs with sensitive information, it might incite or manipulate public opinion.
To mitigate the potential problems, illegal data collection should be prevented and it is encouraged to put the dataset under rigorous scrutiny before the release.
% In this paper, we address the problem of weak-generalization of Graph Neural Networks. We study augmentation for GNNs on graph-structured data, so we have some issues that graph-structured data and GNNs intrinsically have. Since graph data is provided by a certain community, it should be noted that the data itself might be biased depending on the community. In addition, since GNNs use surrounding neighbors' information in the process of aggregation, there may be security issues of data privacy such as their relationship and the property. 

\paragraph{Limitations.} Since we adopt the MCMC sampling for augmentation, our method also has the burn-in issue that is common in MCMC methods. To mitigate this problem, we start from the original graph which is at an area with a high probability density. But, for an extreme target distribution, this initialization might not be sufficient to resolve the burn-in issue and better initialization needs to be studied. 
In addition, we propose a simple target distribution based on Gaussian distribution with a normalization. However, there might be more ideal target distributions for effective augmentation. These are left for future works.
