# Supplementary material for: Metropolis-Hastings Data Augmentation for Graph Neural Networks
Source: arXiv:2203.14082 source file (2022-03-26)
Supplement: Supplementary file 15 [file appendix_ablation.tex]

\begin{table}[ht] 
  \caption{Ablation study of MH-Aug with GCN.} \label{table:ablation}
  \centering
\setlength{\tabcolsep}{6pt}

\begin{adjustbox}{width=1.0\textwidth}    
  \begin{tabular}{l|ccccc}
    \toprule
    % \multicolumn{7}{c}{asd}\\
    \textbf{Methods} & \textbf{CORA} & \textbf{CITESEER} & \textbf{Computers} & \textbf{Photo} & \textbf{CS}\\
    \midrule
    
    % \multirow{3}{*}{}
    Vanilla & 81.54{\scriptsize$\pm$0.76} & 71.64{\scriptsize$\pm$0.31} & 79.68{\scriptsize$\pm$2.16} & 89.02{\scriptsize$\pm$1.49} & 91.45{\scriptsize$\pm$0.28} \\
    MH-Aug (w/o Reg) & 83.55{\scriptsize$\pm$0.34} & 72.96{\scriptsize$\pm$0.48} & 80.95{\scriptsize$\pm$2.03} & 89.65{\scriptsize$\pm$1.67} & 91.81{\scriptsize$\pm$0.33} \\
    MH-Aug (w/o Normalization)  & 82.88{\scriptsize$\pm$0.62} & 74.81{\scriptsize$\pm$0.48} & 73.49{\scriptsize$\pm$2.20} & 90.75{\scriptsize$\pm$1.41} & 92.45{\scriptsize$\pm$0.62} \\
    MH-Aug (w/o Entropy)  & 82.53{\scriptsize$\pm$0.49} & 71.63{\scriptsize$\pm$0.57} & 80.88{\scriptsize$\pm$1.90} & 89.82{\scriptsize$\pm$1.63} & 91.96{\scriptsize$\pm$0.60} \\
    MH-Aug & \textbf{85.16{\scriptsize$\pm$0.35}} & \textbf{75.49{\scriptsize$\pm$0.29}} & \textbf{82.80{\scriptsize$\pm$2.08}} & \textbf{90.87{\scriptsize$\pm$1.49}} & \textbf{92.60{\scriptsize$\pm$0.43}} \\
    
    \bottomrule
  \end{tabular}
\end{adjustbox}
\vspace{-5pt}
\end{table}
