# Supplementary material for: Metropolis-Hastings Data Augmentation for Graph Neural Networks
Source: arXiv:2203.14082 source file (2022-03-26)
Supplement: Supplementary file 16 [file appendix_lar.tex]

\begin{table}[h] 
  \caption{Node classification results on large datasets with K labeled data per class.} \label{table:large}
  \centering
  \label{ablation2}
\begin{adjustbox}{width=11cm}     
\begin{tabular}{cl|cccc}
\toprule
\multirow{2}{*}{\textbf{BaseGNNs}} & \multirow{2}{*}{\textbf{Method}} &  \multicolumn{2}{c}{\textbf{ogbn-arxiv}} &  \multicolumn{2}{c}{\textbf{CORA Full}} \\
% \cmidrule{3-4}
 &  & K=10 & K=20 & K=10 & K=20\\
\midrule
\multirow{2}{*}{\textbf{GCN}}
& Vanilla   & 47.83{\scriptsize$\pm$1.13} & 54.17{\scriptsize$\pm$1.80} & 54.14{\scriptsize$\pm$ 0.72} & 59.99{\scriptsize$\pm$ 0.39}  \\
& MH-Aug & \textbf{56.19{\scriptsize$\pm$0.44}} & \textbf{61.22{\scriptsize$\pm$0.33}}& \textbf{56.27{\scriptsize$\pm$1.97}} & \textbf{62.79{\scriptsize$\pm$0.49}}   \\
\midrule
\multirow{2}{*}{\textbf{GraphSAGE}}
& Vanilla  & 42.35{\scriptsize$\pm$1.52} & 49.19{\scriptsize$\pm$0.42}  & 52.31{\scriptsize$\pm$ 1.18} & 58.85{\scriptsize$\pm$ 0.43}  \\
& MH-Aug & \textbf{59.01{\scriptsize$\pm$0.28}} & \textbf{61.09{\scriptsize$\pm$0.67}} & \textbf{52.46{\scriptsize$\pm$0.88}} & \textbf{62.57{\scriptsize$\pm$0.73}}  \\

\bottomrule
\end{tabular}
\end{adjustbox}

\end{table}
